# Supplementary material for: Gunrock 2.0: A User Adaptive Social Conversational System
Source: arXiv:2011.08906 source file (2020-11-30)
Supplement: Supplementary file 1 [file ap_2020.tex]

\documentclass{article}

% if you need to pass options to natbib, use, e.g.:
% \PassOptionsToPackage{numbers, compress}{natbib}
% before loading ap_2017
%
% to avoid loading the natbib package, add option nonatbib:
% \usepackage[nonatbib]{ap_2017}

% to compile a camera-ready version, add the [final] option, e.g.:
%\usepackage[final]{ap_2017}
\usepackage{ap_2017}

\usepackage[utf8]{inputenc} % allow utf-8 input
\usepackage[T1]{fontenc}    % use 8-bit T1 fonts
\usepackage{hyperref}       % hyperlinks
\usepackage{url}            % simple URL typesetting
\usepackage{booktabs}       % professional-quality tables
\usepackage{amsfonts}       % blackboard math symbols
\usepackage{nicefrac}       % compact symbols for 1/2, etc.
\usepackage{microtype}      % microtypography

\title{Formatting instructions for Alexa Prize 2017}

% The \author macro works with any number of authors. There are two
% commands used to separate the names and addresses of multiple
% authors: \And and \AND.
%
% Using \And between authors leaves it to LaTeX to determine where to
% break the lines. Using \AND forces a line break at that point. So,
% if LaTeX puts 3 of 4 authors names on the first line, and the last
% on the second line, try using \AND instead of \And before the third
% author name.

\author{
	David S.~Hippocampus\thanks{Use footnote for providing further
		information about author (webpage, alternative
		address)---\emph{not} for acknowledging funding agencies.} \\
	Department of Computer Science\\
	Cranberry-Lemon University\\
	Pittsburgh, PA 15213 \\
	\texttt{hippo@cs.cranberry-lemon.edu} \\
	\and
	Coauthor \\
	Affiliation \\
	Address \\
	\texttt{email} \\
	\and
	Coauthor \\
	Affiliation \\
	Address \\
	\texttt{email} \\
	\and
	Coauthor \\
	Affiliation \\
	Address \\
	\texttt{email} \\
	\and
	Coauthor \\
	Affiliation \\
	Address \\
	\texttt{email} \\
}

\begin{document}

\maketitle

\begin{abstract}
  The abstract paragraph should be indented \nicefrac{1}{2}~inch
  (3~picas) on both the left- and right-hand margins. Use 10~point
  type, with a vertical spacing (leading) of 11~points.  The word
  \textbf{Abstract} must be centered, bold, and in point size 12. Two
  line spaces precede the abstract. The abstract must be limited to
  one paragraph.
\end{abstract}

\section{Submission of papers to Alexa Prize 2017}
The Alexa Prize requires electronic submissions. The electronic submission site is

\begin{center}
s3://alexaprize/<team-account-number>/<team-account-number>.pdf
\end{center}

\subsection{Retrieval of style files}

The style files for Alexa Prize are based on the NIPS format. Original NIPS format files are available at:

\begin{center}
  \url{http://www.nips.cc/}
\end{center}

At submission time, please omit the \verb+final+ option. This will
anonymize your submission and add line numbers to aid review.  Please
do \emph{not} refer to these line numbers in your paper as they will
be removed during generation of camera-ready copies.

The file \verb+ap_2017.tex+ may be used as a ``shell'' for writing
your paper. All you have to do is replace the author, title, abstract,
and text of the paper with your own.

The formatting instructions contained in these style files are
summarized in Sections \ref{gen_inst}, \ref{headings}, and
\ref{others} below.

\section{General formatting instructions}
\label{gen_inst}

The text must be confined within a rectangle 5.5~inches (33~picas)
wide and 9~inches (54~picas) long. The left margin is 1.5~inch
(9~picas).  Use 10~point type with a vertical spacing (leading) of
11~points.  Times New Roman is the preferred typeface throughout, and
will be selected for you by default.  Paragraphs are separated by
\nicefrac{1}{2}~line space (5.5 points), with no indentation.

The paper title should be 17~point, initial caps/lower case, bold,
centered between two horizontal rules. The top rule should be 4~points
thick and the bottom rule should be 1~point thick. Allow
\nicefrac{1}{4}~inch space above and below the title to rules. All
pages should start at 1~inch (6~picas) from the top of the page.

For the final version, authors' names are set in boldface, and each
name is centered above the corresponding address. The lead author's
name is to be listed first (left-most), and the co-authors' names (if
different address) are set to follow. If there is only one co-author,
list both author and co-author side by side.

Please pay special attention to the instructions in Section \ref{others}
regarding figures, tables, acknowledgments, and references.

\section{Headings: first level}
\label{headings}

All headings should be lower case (except for first word and proper
nouns), flush left, and bold.

First-level headings should be in 12-point type.

\subsection{Headings: second level}

Second-level headings should be in 10-point type.

\subsubsection{Headings: third level}

Third-level headings should be in 10-point type.

\paragraph{Paragraphs}

There is also a \verb+\paragraph+ command available, which sets the
heading in bold, flush left, and inline with the text, with the
heading followed by 1\,em of space.

\section{Citations, figures, tables, references}
\label{others}

These instructions apply to everyone.

\subsection{Citations within the text}

The \verb+natbib+ package will be loaded for you by default.
Citations may be author/year or numeric, as long as you maintain
internal consistency.  As to the format of the references themselves,
any style is acceptable as long as it is used consistently.

The documentation for \verb+natbib+ may be found at
\begin{center}
  \url{http://mirrors.ctan.org/macros/latex/contrib/natbib/natnotes.pdf}
\end{center}
Of note is the command \verb+\citet+, which produces citations
appropriate for use in inline text.  For example,
\begin{verbatim}
   \citet{hasselmo} investigated\dots
\end{verbatim}
produces
\begin{quote}
  Hasselmo, et al.\ (1995) investigated\dots
\end{quote}

If you wish to load the \verb+natbib+ package with options, you may
add the following before loading the \verb+ap_2017+ package:
\begin{verbatim}
   \PassOptionsToPackage{options}{natbib}
\end{verbatim}

If \verb+natbib+ clashes with another package you load, you can add
the optional argument \verb+nonatbib+ when loading the style file:
\begin{verbatim}
   \usepackage[nonatbib]{ap_2017}
\end{verbatim}

As submission is double blind, refer to your own published work in the
third person. That is, use ``In the previous work of Jones et
al.\ [4],'' not ``In our previous work [4].'' If you cite your other
papers that are not widely available (e.g., a journal paper under
review), use anonymous author names in the citation, e.g., an author
of the form ``A.\ Anonymous.''

\subsection{Footnotes}

Footnotes should be used sparingly.  If you do require a footnote,
indicate footnotes with a number\footnote{Sample of the first
  footnote.} in the text. Place the footnotes at the bottom of the
page on which they appear.  Precede the footnote with a horizontal
rule of 2~inches (12~picas).

Note that footnotes are properly typeset \emph{after} punctuation
marks.\footnote{As in this example.}

\subsection{Figures}

All artwork must be neat, clean, and legible. Lines should be dark
enough for purposes of reproduction. The figure number and caption
always appear after the figure. Place one line space before the figure
caption and one line space after the figure. The figure caption should
be lower case (except for first word and proper nouns); figures are
numbered consecutively.

You may use color figures.  However, it is best for the figure
captions and the paper body to be legible if the paper is printed in
either black/white or in color.
\begin{figure}[h]
  \centering
  \fbox{\rule[-.5cm]{0cm}{4cm} \rule[-.5cm]{4cm}{0cm}}
  \caption{Sample figure caption.}
\end{figure}

\subsection{Tables}

All tables must be centered, neat, clean and legible.  The table
number and title always appear before the table.  See
Table~\ref{sample-table}.

Place one line space before the table title, one line space after the
table title, and one line space after the table. The table title must
be lower case (except for first word and proper nouns); tables are
numbered consecutively.

Note that publication-quality tables \emph{do not contain vertical
  rules.} We strongly suggest the use of the \verb+booktabs+ package,
which allows for typesetting high-quality, professional tables:
\begin{center}
  \url{https://www.ctan.org/pkg/booktabs}
\end{center}
This package was used to typeset Table~\ref{sample-table}.

\begin{table}[t]
  \caption{Sample table title}
  \label{sample-table}
  \centering
  \begin{tabular}{lll}
    \toprule
    \multicolumn{2}{c}{Part}                   \\
    \cmidrule{1-2}
    Name     & Description     & Size ($\mu$m) \\
    \midrule
    Dendrite & Input terminal  & $\sim$100     \\
    Axon     & Output terminal & $\sim$10      \\
    Soma     & Cell body       & up to $10^6$  \\
    \bottomrule
  \end{tabular}
\end{table}

\section{Final instructions}

Do not change any aspects of the formatting parameters in the style
files.  In particular, do not modify the width or length of the
rectangle the text should fit into, and do not change font sizes
(except perhaps in the \textbf{References} section; see below). Please
note that pages should be numbered.

\section{Preparing PDF files}

Please prepare submission files with paper size ``US Letter,'' and
not, for example, ``A4.''

Fonts were the main cause of problems in the past years. Your PDF file
must only contain Type 1 or Embedded TrueType fonts. Here are a few
instructions to achieve this.

\begin{itemize}

\item You should directly generate PDF files using \verb+pdflatex+.

\item You can check which fonts a PDF files uses.  In Acrobat Reader,
  select the menu Files$>$Document Properties$>$Fonts and select Show
  All Fonts. You can also use the program \verb+pdffonts+ which comes
  with \verb+xpdf+ and is available out-of-the-box on most Linux
  machines.

\item The IEEE has recommendations for generating PDF files whose
  fonts are also acceptable for Alexa Prize. Please see
  \url{http://www.emfield.org/icuwb2010/downloads/IEEE-PDF-SpecV32.pdf}

\item \verb+xfig+ "patterned" shapes are implemented with bitmap
  fonts.  Use "solid" shapes instead.

\item The \verb+\bbold+ package almost always uses bitmap fonts.  You
  should use the equivalent AMS Fonts:
\begin{verbatim}
   \usepackage{amsfonts}
\end{verbatim}
followed by, e.g., \verb+\mathbb{R}+, \verb+\mathbb{N}+, or
\verb+\mathbb{C}+ for $\mathbb{R}$, $\mathbb{N}$ or $\mathbb{C}$.  You
can also use the following workaround for reals, natural and complex:
\begin{verbatim}
   \newcommand{\RR}{I\!\!R} %real numbers
   \newcommand{\Nat}{I\!\!N} %natural numbers
   \newcommand{\CC}{I\!\!\!\!C} %complex numbers
\end{verbatim}
Note that \verb+amsfonts+ is automatically loaded by the
\verb+amssymb+ package.

\end{itemize}

If your file contains type 3 fonts or non embedded TrueType fonts, we
will ask you to fix it.

\subsection{Margins in \LaTeX{}}

Most of the margin problems come from figures positioned by hand using
\verb+\special+ or other commands. We suggest using the command
\verb+\includegraphics+ from the \verb+graphicx+ package. Always
specify the figure width as a multiple of the line width as in the
example below:
\begin{verbatim}
   \usepackage[pdftex]{graphicx} ...
   \includegraphics[width=0.8\linewidth]{myfile.pdf}
\end{verbatim}
See Section 4.4 in the graphics bundle documentation
(\url{http://mirrors.ctan.org/macros/latex/required/graphics/grfguide.pdf})

A number of width problems arise when \LaTeX{} cannot properly
hyphenate a line. Please give LaTeX hyphenation hints using the
\verb+\-+ command when necessary.

\subsubsection*{Acknowledgments}

Use unnumbered third level headings for the acknowledgments. All
acknowledgments go at the end of the paper. Do not include
acknowledgments in the anonymized submission, only in the final paper.

\section*{References}

References follow the acknowledgments. Use unnumbered first-level
heading for the references. Any choice of citation style is acceptable
as long as you are consistent. It is permissible to reduce the font
size to \verb+small+ (9 point) when listing the references. {\bf
  Remember that you can use a ninth page as long as it contains
  \emph{only} cited references.}
\medskip

\small

[1] Alexander, J.A.\ \& Mozer, M.C.\ (1995) Template-based algorithms
for connectionist rule extraction. In G.\ Tesauro, D.S.\ Touretzky and
T.K.\ Leen (eds.), {\it Advances in Neural Information Processing
  Systems 7}, pp.\ 609--616. Cambridge, MA: MIT Press.

[2] Bower, J.M.\ \& Beeman, D.\ (1995) {\it The Book of GENESIS:
  Exploring Realistic Neural Models with the GEneral NEural SImulation
  System.}  New York: TELOS/Springer--Verlag.

[3] Hasselmo, M.E., Schnell, E.\ \& Barkai, E.\ (1995) Dynamics of
learning and recall at excitatory recurrent synapses and cholinergic
modulation in rat hippocampal region CA3. {\it Journal of
  Neuroscience} {\bf 15}(7):5249-5262.

\end{document}
