# Supplementary material for: Gunrock 2.0: A User Adaptive Social Conversational System
Source: arXiv:2011.08906 source file (2020-11-30)
Supplement: Supplementary file 2 [file appendix.tex]

\appendix 
\section{Appendix} \label{appendix}
% \import{appendix/}{dialog_act.tex} 
\subsection{Intent scheme} \label{appendix-intent-scheme}
